# Supplementary material for: Observation of anomalous diffusion and fractional self-similarity in one dimension
Source: arXiv:1109.1503 source file (2012-03-02)
Supplement: Supplementary file 1 [file supplementary_material.pdf]

# Supplementary material for the manuscript "Observation of anomalous diffusion and fractional self-similarity in one dimension"

Yoav Sagi, Miri Brook, Ido Almog, and Nir Davidson

*Department of Physics of Complex Systems,*

*Weizmann Institute of Science, Rehovot 76100, Israel*

In the following document we provide more details regarding the numerical simulations presented in the main text.

## MONTE-CARLO WAVE FUNCTIONS SIMULATIONS

Though diffusion is a classical phenomenon, the full understanding of our apparatus requires a quantum mechanical simulation which includes the interaction of the atoms with the light field. To that end we have written a Monte Carlo Wave-Functions simulation (MCWF) of laser cooling of non-interacting two-level atoms in one dimensional optical molasses [1, 2]. We simulate an angular momentum $J_g = 1/2$ to $J_e = J_g + 1 = 3/2$ transitions induced by two counter propagating laser beams, with linear and orthogonal polarization ($lin \perp lin$ configuration), which creates a position-dependent polarization field and can be treated as periodic potential of depth $U_0$. This potential depends on the laser parameters and on the atom-laser interaction term [3]. We simulate the Hamiltonian evolution of a single atomic wave function by propagating it both in real and momentum space using the split-step technique [4]. The Hamiltonian evolution is "interrupted" by spontaneous photon scattering described by the quantum jump approach [5]. The potential depth is controlled by the laser power and its detuning, $\delta$, from the atomic line width, $\gamma$. The diffusion process is analyzed for different potential depths, starting from the point in which the velocity distribution had reached steady state. This time is denoted by $t_{ss}$ and it depends on the potential depth. The length of the simulated evolution is of the order of $10t_{ss} \sim 1000\gamma^{-1}$.

There are two important differences between the experiment and our simulations which are introduced to simplify and facilitate the numerics. First, in the simulation we take into account only two internal low-energy states, as apposed to the real multi level $^{87}Rb$ atoms. Second, in the simulation we set $\delta = -\gamma$ and vary the potential depth by changing the laser power. Working with the experimental value of $\delta$ was computationally too demanding for our resources. Despite these differences, the simulation provides a fine qualitative description of the experiment, as shown in the figures below.

In Fig. 1 we plot on a log-log scale the full width at half the maximum (FWHM) as function of time. Similarly to the experiment, we find that the width increases as a power-law with time. The resulting linear slope is the dynamical diffusion exponent $\alpha$, as discussed in the text. There is a numerical discrepancy between the potential depths in the simulation

and in the experiment, which is expected due to the differences explained before.

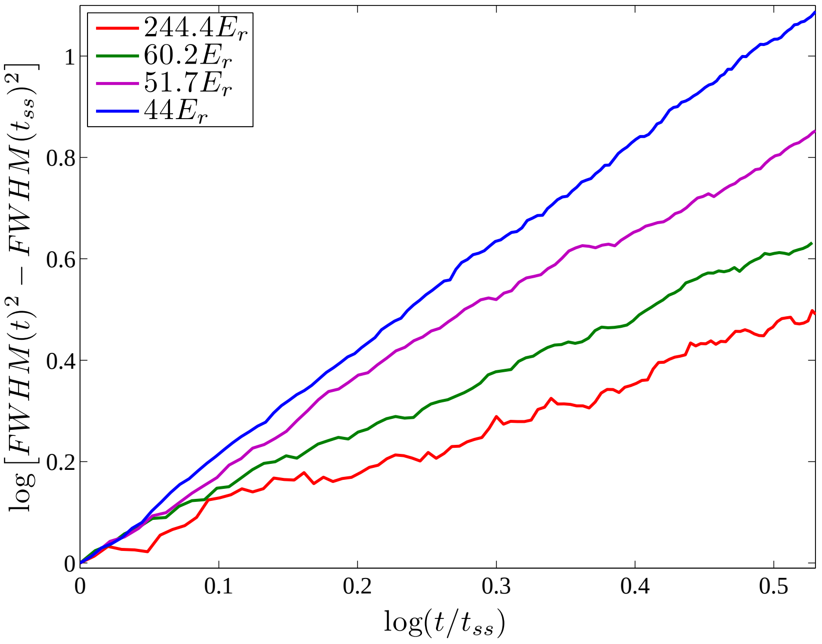


FIG. 1. Normalized squared mean displacement is plotted vs. time, on a logarithmic scale, represented by circles. $t_{ss}$ stands for the time at which the momentum distribution had reached steady state, and the point in which we begin to analyze the absolute mean displacement. Each color corresponds to evolution in a different potential depth.

The simulation also enables us to study the shape of the spatial distribution. In general, we find very high resemblance comparing the parameters deduce from the experiment with the simulated ones, such as the distribution functional shape, its temporal evolution and its dependence on potential depth, the self similarity measure dependence on $\alpha$ and the variation in minimum position with potential depth. In Fig. 2 we plot the distributions at different times for a $U_0 = 44.5E_R$ lattice. The data collapses to the same curve when both axes are re-scaled according to Eq. 2 in the text, as shown in Fig. 2. We further investigate the self-similarity in Fig. 3 where the measure $m(\alpha)$ (see text for the definition) is depicted for three potential depths. The shape of these curves is similar to the one obtained from the experimental data.

Motivated by the experimental findings, we use the Lévy distribution as fitting functions

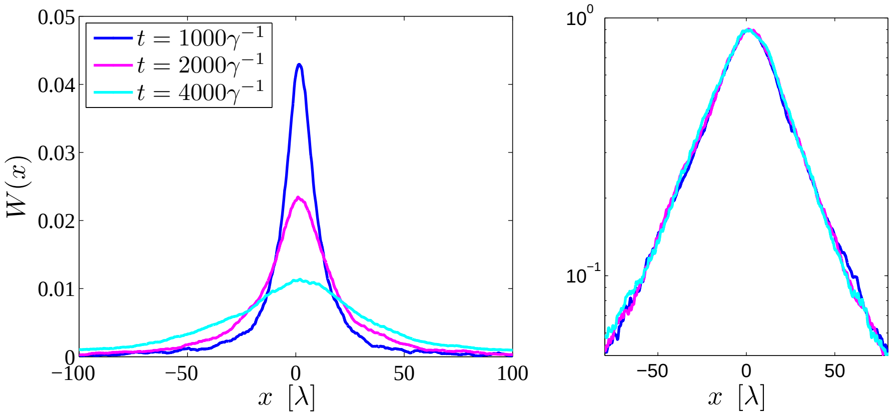


FIG. 2. (a)Atomic spatial distribution of $N = 2500$ atoms, at $t = 1000, 2000, 4000\gamma^{-1}$ in potential depth $U_0 = 44.5E_R$. The distribution becomes broader at larger times, as expected in diffusion process. (b) The rescaled distributions with $\alpha = 1.12$ on a semi log scale which emphasizes their power law tail.

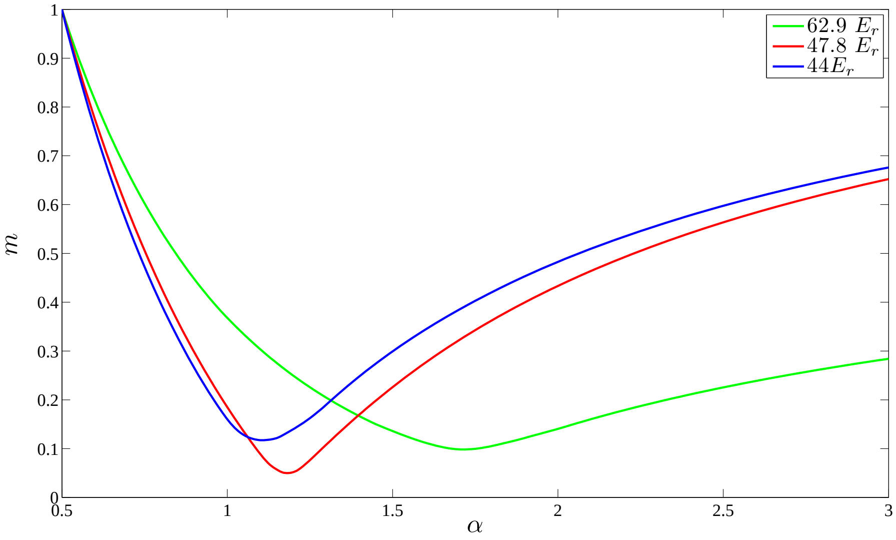


FIG. 3. The measure of self-similarity as function of the diffusion exponent $\alpha$, for different potential depths. Each point is obtained from 30 distributions taken at $t_n = 80n\gamma^{-1}$, where $n = 1, 2, .., 30$. The first encountered distribution is taken at $t_1 = t_{ss}$.

(Fig. 4). We find that they fit very well the simulation results. We also find that the extracted Lévy exponent for a certain lattice depth is the same for times larger than $t_{ss}$ with an accuracy of 0.1%.

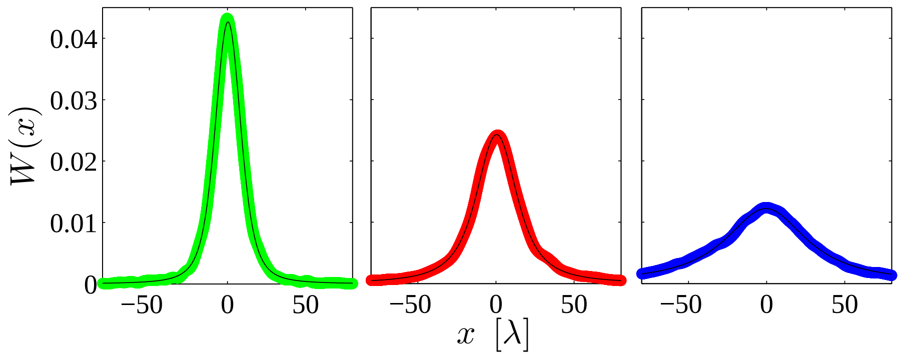


FIG. 4. Spatial distribution at $t = 2000\gamma^{-1}$ and the fit to Levy function, in lattices of $88E_R$, $62.8E_R$, $48.9E_R$, from left to right respectively.

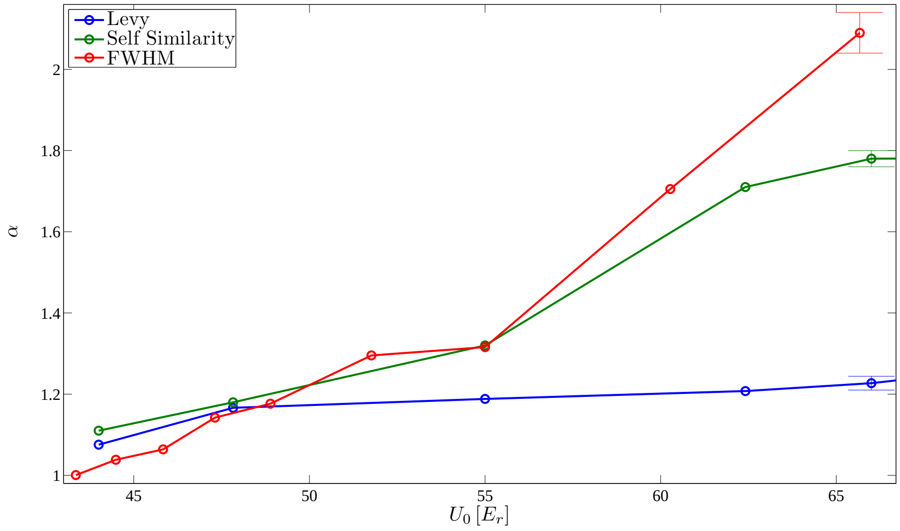


FIG. 5. The diffusion exponent $\alpha$ as a function of the lattice depth. Similar to figure 3 in the text, the exponent is extracted by three different methods: fitting the FWHM data at different times to a power-law (red), from the measure of the self-similar transformation (green), and by fitting the distributions with a Lévy $L_\alpha$ function (blue).

Finally, in Fig. 5 we compare between the exponents extracted from the dynamics of the FWHM, the best-fitted Lévy distribution and the self-similarity measure. The results of the simulation show a similar trend as the experiment: in deep potentials, the best-fitted Lévy exponents are of lower value then the dynamical exponents and the self-similarity measure. A benefit of of the MCWF simulation is that it provides us with a *single* atomic trajectory

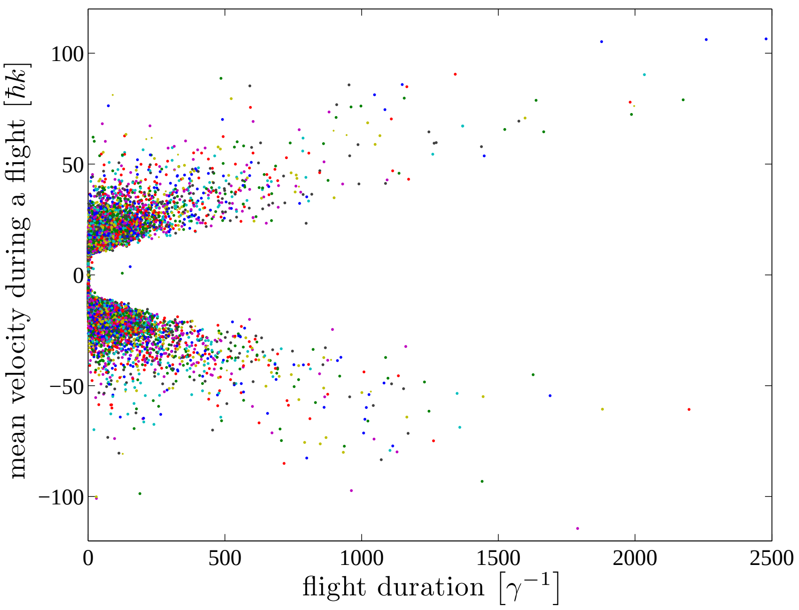


FIG. 6. The mean velocity during a flight is plotted as function of the flight duration. Each point represents a single flight event of 3000 simulated particles. The different colors correspond to different particles. Each particle experience 4 flights on average during its evolution in lattice of $U_0 = 45E_r$, up to the final simulated time of $2500\gamma^{-1}$.

rather then ensemble average. As long as the jump operators describes correctly the collapse events in the experiment, we can attribute these single trajectories a physical reality and use them to extract single-particle properties in the process. In order to explain the discrepancy found between the Lévy and the dynamical exponent in deep potentials, we examine the correlations between the atom's velocity during a flight (a flight is defined such that the total energy of the atom is larger then the potential depth) and the duration of the flight. Fig. 6 clearly shows the existence of this correlation; as the flight duration is longer it is more likely to find that the atom's velocity during this flight is higher.

## CLASSICAL SIMULATIONS OF ANOMALOUS DIFFUSION

A simple but powerful tool in studying diffusion processes is a classical Monte-Carlo simulation. The simulation calculates the trajectory of many particles which move and occasionally change their velocity. The motion of each particle is modeled by a succession

of steps, each composed of two stages: a waiting stage in which the particle is trapped in a particular lattice site and does not move, and a flight stage in which it moves at some velocity. For each particle and in each step of the simulation, three variables are drawn: the waiting time, the flight duration and the particle's velocity. We typically simulate the trajectories of 10000 particles to obtain the spatial distribution after different diffusion times. Similarly to the experiment, we extract the shape exponent by fitting the simulated distribution to a Lévy distribution and the dynamical exponent by fitting the time-evolution of the width to a power-law (starting after 10 steps to avoid the initial short "ballistic" enpension). In what follows we refer to these exponents as $\alpha_{shape}$ and $\alpha_{dynamical}$, respectively. The distribution of each of these three variables (waiting time, flight time and velocity) is assumed to be Levy stable distributions. This is done since these distributions are very general in nature and are simply characterized by three characteristic exponents: $\alpha_{velocity}$,$\alpha_{waiting}$ and $\alpha_{flights}$.

In Fig. 7 we depict the end result of a simulation with $\alpha_{flights} = 1.5$ and $\alpha_{velocity} = \alpha_{waiting} = 2$, and the corresponding fit to a Lévy distribution. In this particular case, since $\alpha_{waiting} = 2$ the diffusion process is described by the fractional diffusion equation (FDE) with $\beta = 1, \mu = 1.5$, and therefore we expect the Lévy distribution to be an exact solution [6]. Indeed, the fit to a Lévy distribution produces an r-square of 0.99. The value of the Lévy characteristic exponent is found to be 1.58, very close to the predicted value of 1.5.

In Table I we enlist other results of the simulation with different exponents for the various distributions (here it is assumed that there are no correlations between the variables). The first two rows show that having heavy tailed distribution with a diverging second moment for the flight duration or velocities has a similar effect. In both cases we obtain the result expected from the FDE, namely that the dynamical and shape exponents are very similar, and their value is very close to $\mu$.

The third row gives the results for a waiting times distribution with a diverging first moment. This case corresponds to $\beta < 1$ in the FDE, for which the solutions are not anymore the Lévy functions. We indeed observe that a cusp develops at $x = 0$ and the fit to Lévy distribution is not as good as for $\beta = 1$. Nevertheless, even in this case the fits to the Lévy functions are surprisingly good, producing typical r-square values larger than 0.95. Moreover, in both the experiment and simulation we are limited by signal to noise or particle number so the distribution tail behavior is only resolved at a limited range. It is therefore meaningful to use the Lévy distribution as a fitting function in this range, even

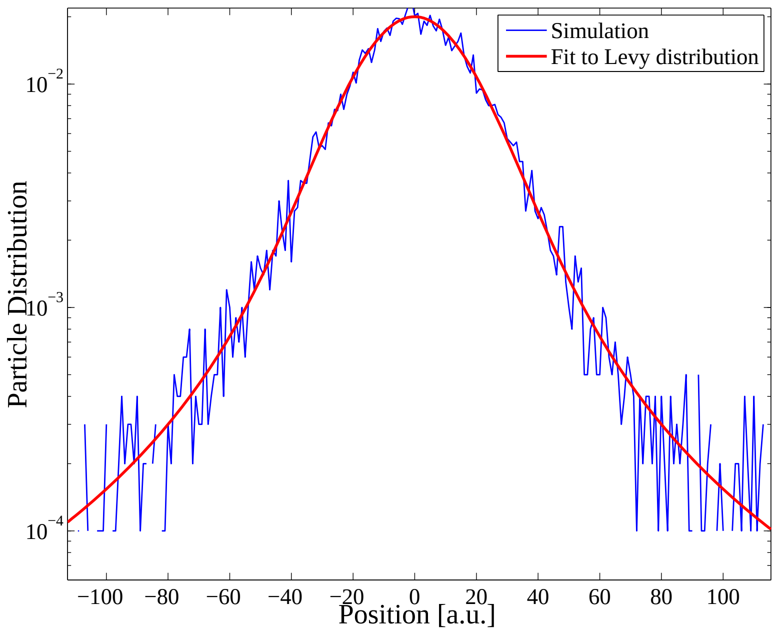


FIG. 7. The probability distribution as calculated by the classical simulation with 10,000 particles after an average of 38 steps, with $\alpha_{flight} = 1.5$ and $\alpha_{velocity} = \alpha_{waiting} = 2$. The red line is a fit to a Lévy distribution which yields $\alpha_{shape} = 1.58$.

though its asymptotic scaling is different than the exact solution.

As mentioned in the text, the dynamical exponent is predicted to be $\mu/\beta$, where $\mu$ and $\beta$ are the parameters in the FDE. As can be seen in the third row in the table, for the case $\alpha_{waiting} = 0.8$ and $\alpha_{flights} = \alpha_{velocities} = 2$, which corresponds to $\beta = 0.8$ and $\mu = 2$, we recover this result. This set of parameters reveals another interesting fact: when fitting the case of $\beta < 1$ by a Lévy distribution, the shape exponent may be smaller than the dynamical exponent. Since in the experiment the dynamical exponent is smaller than 2, the parameters in the simulations need to satisfy $\mu < 2\beta$. The forth row in the table gives an example of a set which produces results similar to the experimental observations. However, as the lattice depth increases, so does the exponent of the velocity distribution [7]. The simulation shows that for increasing $\alpha_{velocity}$, the fitted shape exponent becomes larger than 1, in contrast to the experiment. For example, the fifth row shown that for $\alpha_{velocity} = 1.3$ we could only get $\alpha_{shape} \approx 0.9$, and already for $\alpha_{velocity} = 1.6$ (the sixth row in the table) we can not obtain $\alpha_{shape} > 1$.

| # | $\alpha_{velocity}$ | $\alpha_{waiting}$ | $\alpha_{flights}$ | $\alpha_{shape}$ | $\alpha_{dynamical}$ |
|---|---|---|---|---|---|
| 1 | 1.5 | 2 | 2 | 1.44 | 1.48 |
| 2 | 2 | 2 | 1.5 | 1.6 | 1.55 |
| 3 | 2 | 0.8 | 2 | 1.51 | 2.5 |
| 4 | 1.1 | 0.7 | 2 | 0.72 | 1.58 |
| 5 | 1.3 | 0.7 | 2 | 0.91 | 1.9 |
| 6 | 1.6 | 0.805 | 2 | 1.25 | 1.98 |
| 7 | 1.7 | 0.8 | 1.7 | 1.21 | 1.97 |

TABLE I. Results of the classical simulation for different velocity, waiting time and flight duration distributions without correlations. The extracted dynamical and shape exponents has a typical 2% accuracy.

The MCWF simulations clearly show that correlations between the flight duration and velocity exist. Therefore, we set to test whether this fact can better account for the experimental observations. For this purpose we use the same classical simulation, but this time introduce correlations between the velocity and flight duration. The simplest way to do so is to assume that they are proportional to one another. In other words, we draw a velocity for a particle, $v$, and assume that the flight duration is given by $cv$, where $c$ has the correct units (in the simulation it is set to unity). We find that such correlations together with $\beta < 1$ can explain the experimental observations very well, even for high $\alpha_{velocity}$. For example, for $\alpha_{velocity} = 1.7$ and $\alpha_{waiting} = 0.8$ we find $\alpha_{dynamical} = 1.41$ and $\alpha_{shape} = 0.77$. For comparison, the result for the same characteristic exponents without correlations is shown in the last row of Table I, where we find that $\alpha_{shape} > 1$. Note that $\alpha_{waiting} = 0.8$ is a typical value we find in the MCWF simulations.


[1] K. Mølmer, Y. Castin, and J. Dalibard, J. Opt. Soc. Am. B **10**, 524 (1993).

[2] S. Marksteiner, K. Ellinger, and P. Zoller, Physical Review A **53**, 3409 (1996).

[3] Y. Castin and K. Mølmer, Phys. Rev. Lett. **74**, 3772 (1995).

[4] J. A. C. Weideman and B. M. Herbst, SIAM Journal on Numerical Analysis **23**, pp. 485 (1986).

[5] Y. Castin and J. Dalibard, EPL (Europhysics Letters) **14**, 761 (1991).

[6] R. Metzler and J. Klafter, Physics Reports **339**, 1 (2000).

[7] Y. Castin, J. Dalibard, and C. Cohen-Tannoudji, "Light induced kinetic effects on atoms, ions, and molecules," (ETS Editrice, 1991) Chap. The limits of Sisyphus cooling.
